# Supplementary material for: Observation of a dispersive charge mode in hole-doped cuprates using resonant inelastic x-ray scattering at the oxygen K edge
Source: arXiv:1703.01018 ancillary file (2017-03-03)
Supplement: Supplementary file 1 [file SupplementalMaterial.pdf]

# Supplemental Material

# Observation of a dispersive charge mode in hole-doped cuprates using resonant inelastic x-ray scattering at the oxygen $K$ edge

K. Ishii,[1] T. Tohyama,[2] S. Asano,[3] K. Sato,[3] M. Fujita,[3] S. Wakimoto,[4] K. Tustsui,[1] S. Sota,[5] J. Miyawaki,[6] H. Niwa,[6] Y. Harada,[6] J. Pelliciari,[7,*] Y. Huang,[7] T. Schmitt,[7] Y. Yamamoto,[8] and J. Mizuki[8]

[1]*Synchrotron Radiation Research Center, National Institutes for Quantum and Radiological Science and Technology, Hyogo 679-5148, Japan*
[2]*Department of Applied Physics, Tokyo University of Science, Tokyo 125-8585, Japan*
[3]*Institute for Materials Research, Tohoku University, Sendai 980-8577, Japan*
[4]*Materials Science Research Center, Japan Atomic Energy Agency, Ibaraki 319-1195, Japan*
[5]*Computational Materials Science Research Team, RIKEN Advanced Institute for Computational Science (AICS), Kobe, Hyogo 650-0047, Japan*
[6]*Institute for Solid State Physics, University of Tokyo, Chiba 277-8581, Japan*
[7]*Research Department Synchrotron Radiation and Nanotechnology, Paul Scherrer Institut, CH-5232 Villigen PSI, Switzerland*
[8]*Graduate School of Science and Technology, Kwansei Gakuin University, Hyogo 669-1337, Japan*

(Dated: March 3, 2017)

## S1. MOMENTUM DEPENDENCE OF TWO-MAGNON EXCITATIONS

The momentum-dependent two-magnon excitations are calculated for the $t$-$t'$-$t''$-$J$ model with three-site term. The Hamiltonian is given by

$$H = H_{tt't''J} + H_{3s}$$

with

$$H_{tt't''J} = -t \sum_{\langle i,j\rangle_{1\mathrm{st}},\sigma} \left(\tilde{c}^{\dagger}_{i,\sigma}\tilde{c}_{j,\sigma} + \mathrm{h.c.}\right) - t' \sum_{\langle i,j\rangle_{2\mathrm{nd}},\sigma} \left(\tilde{c}^{\dagger}_{i,\sigma}\tilde{c}_{j,\sigma} + \mathrm{h.c.}\right) - t'' \sum_{\langle i,j\rangle_{3\mathrm{rd}},\sigma} \left(\tilde{c}^{\dagger}_{i,\sigma}\tilde{c}_{j,\sigma} + \mathrm{h.c.}\right) + J \sum_{\langle i,j\rangle_{1\mathrm{st}}} \mathbf{S}_i \cdot \mathbf{S}_j$$

and

$$H_{3\mathrm{s}} = -\frac{J}{4} \sum_{\langle i,j\rangle_{1\mathrm{st}},\langle i,j'\rangle_{1\mathrm{st}},j\neq j',\sigma} \left(\tilde{c}^{\dagger}_{j',\sigma}\tilde{n}_{i,-\sigma}\tilde{c}_{j,\sigma} - \tilde{c}^{\dagger}_{j',\sigma}\tilde{c}^{\dagger}_{i,-\sigma}\tilde{c}_{i,\sigma}\tilde{c}_{j,-\sigma} + \mathrm{h.c.}\right),$$

where the summations $\langle i,j\rangle_{1\mathrm{st}}$, $\langle i,j\rangle_{2\mathrm{nd}}$, and $\langle i,j\rangle_{3\mathrm{rd}}$ run over first, second, and third nearest-neighbour pairs, respectively. The operator $\tilde{c}_{i,\sigma} = c_{i,\sigma}\left(1 - c^{\dagger}_{i,\sigma}c_{j,\sigma}\right)$ annihilates a localized electron with spin $\sigma$ at site $i$ with the constraint of no double occupancy, and $\mathbf{S}_i$ is the spin operator at site $i$. In the model, we set $t = 1$, $t' = -0.25$, $t'' = 0.12$, and $J = 0.4$. The real value of $t$ in cuprate superconductors is usually taken to be 0.35 eV.

We define the momentum-dependent dynamical two-magnon correlation function as [1]

$$M_{\pm}(\mathbf{q},\omega) = \sum_f \left|\langle f|\, M^{\pm}_{\mathbf{q}}\, |0\rangle\right|^2 \delta\left(\omega - E_f + E_0\right), \quad (1)$$

where $|0\rangle$ and $|f\rangle$ represent the ground state final state with energy $E_0$ and $E_f$, respectively, and $M^{\pm}_{\mathbf{q}} = \sum_{\mathbf{k}} (\cos k_x \pm \cos k_y)\, \mathbf{S}_{\mathbf{k}+\mathbf{q}} \cdot \mathbf{S}_{\mathbf{k}}$. We note that $+$ $(-)$ corresponds to $\mathrm{A}_1$ $(\mathrm{B}_1)$ representation and $\mathbf{S}_{\mathbf{k}} = N^{-1/2} \sum_l e^{-i\mathbf{k}\cdot\mathbf{R}_l}\mathbf{S}_l$ with $\mathbf{R}_l$ being the position vector at site $l$ and $N$ being the total number of sites. Figures 1(a) and (b) show $M_{+}(\mathbf{q},\omega) = M_{\mathrm{A}_1}(\mathbf{q},\omega)$ and $M_{-}(\mathbf{q},\omega) = M_{\mathrm{B}_1}(\mathbf{q},\omega)$, respectively, at $\mathbf{q} = (0.2, 0.1)$

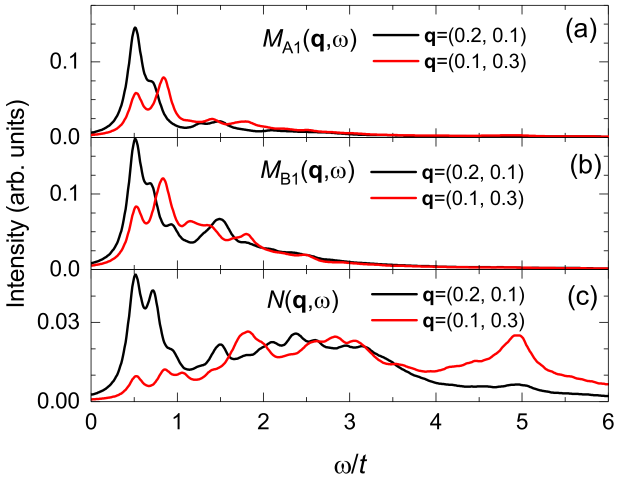


FIG. 1. (Color online) The dynamical two-magnon correlation function for (a) $A_1$ mode, (b) $B_1$ mode, and (c) dynamical charge structure factor at $\mathbf{q} = (0.2, 0.1)$ (black solid line) and $(0.1, 0.3)$ (red solid line) for the $\sqrt{20} \times \sqrt{20}$ periodic cluster of the $t$-$t'$-$t''$-$J$ model with three-site term. $t = 1$, $t' = -0.25$, $t'' = 0.12$, and $J = 0.4$. A Lorentzian broadening with a width of $0.2t$ is used for the spectral weights.

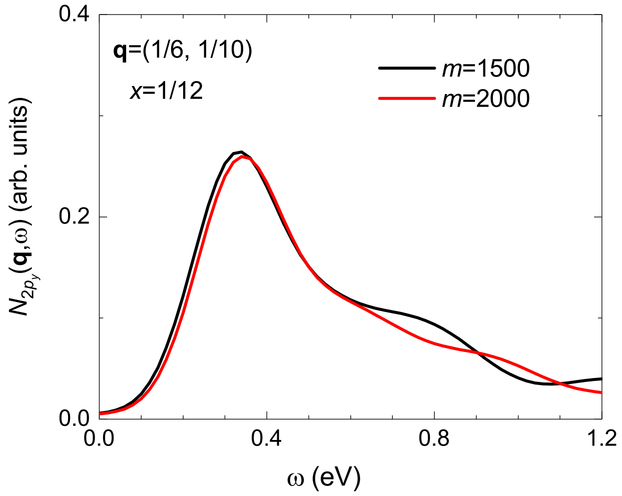


FIG. 2. (Color online) The dependence of $N_{2p_y}(\mathbf{q}, \omega)$ for a given parameter set on the truncation number $m$ in the dynamical DMRG method. A $6 \times 4 = 24$-unit cell $CuO_2$ cluster with cylindrical boundary condition is used. $\mathbf{q} = (6/6, 1/10$. $T_{pp} = 0.3$ eV, $\Delta = 3$ eV, $U_d = 8$ eV, and $U_p = 4$ eV, and hole concentration $x = 1/12$. A Gaussian broadening with a width of 0.1 eV is used for the spectral weights.

and $(0.1, 0.3)$ for a $N = \sqrt{20} \times \sqrt{20}$ periodic cluster with hole concertation $x = 2/20 = 0.1$. We find that the momentum dependence of spectral weight mainly appears only for low-energy region less than $\omega = t = 0.35$ eV. This energy region is smaller than the region more than 0.4 eV where O $K$-edge RIXS has reported a dispersive mode as shown in the main text. For comparison, the dynamical charge structure factor $N(\mathbf{q}, \omega)$ is shown in Fig. 1(c). In contrast to the two-magnon excitations, momentum dependence appears even for high energy region up to $\omega \sim 6t \sim 2$ eV [2]. We note that $\mathbf{q} = (0.2, 0.1)$ and $(0.3, 0.2)$ are nearly upper limit or higher than experimentally accessible momentum transfer.

## S2. DYNAMICAL DMRG CALCULATION OF DYNAMICAL CHARGE STRUCTURE FACTOR IN THE THREE-BAND HUBBAED MODEL

Three-band Hubbard Hamiltonian for the $CuO_2$ plane is given by

$$
\begin{aligned}
H = \sum_{i,\sigma} \Big[ & T_{pd} d^\dagger_{i,\sigma} \left( p_{i+\mathbf{y},\sigma} - p_{i+\mathbf{x},\sigma} - p_{i-\mathbf{y},\sigma} + p_{i-\mathbf{x},\sigma} \right) \\
& + T_{pp} ( p^\dagger_{i+\mathbf{y},\sigma} p_{i+\mathbf{x},\sigma} - p^\dagger_{i-\mathbf{x},\sigma} p_{i+\mathbf{y},\sigma} \\
& \quad + p^\dagger_{i-\mathbf{y},\sigma} p_{i-\mathbf{x},\sigma} - p^\dagger_{i+\mathbf{x},\sigma} p_{i-\mathbf{y},\sigma} ) + \text{h.c.} \Big] \\
& + \Delta \sum_{i,\delta,\sigma} n^p_{i+\delta,\sigma} + U_d \sum_i n^d_{i,\uparrow} n^d_{i,\downarrow} + U_p \sum_{i,\delta} n^p_{i+\delta,\uparrow} n^p_{i+\delta,\downarrow},
\end{aligned}
$$

where the operator $d_{i,\sigma}$ annihilates holes with spin $\sigma$ in $3d_{x^2-y^2}$ orbital at site $i$, $n^d_{i,\sigma} = d^\dagger_{i,\sigma} d_{i,\sigma}$, the $p_{i\pm\mathbf{x}(\mathbf{y}),\sigma}$ are the hole annihilation operators for the $2p_x$ ($2p_y$) orbitals at site $i \pm \mathbf{x}(\mathbf{y})$, $\mathbf{x}$ ($\mathbf{y}$) being the vector connecting neighboring Cu and O ions along the $x$ ($y$) directions, $\delta$ is either $\mathbf{x}$ or $\mathbf{y}$, and $n^p_{i+\delta,\sigma} = p^\dagger_{i+\delta,\sigma} p_{i+\delta,\sigma}$. $T_{pd}$ is the hopping between Cu$3d_{x^2-y^2}$ and O$2p_\sigma$ orbitals, $T_{pp}$ is the hopping between neighboring O$2p_\sigma$ orbitals, $\Delta$ is the charge transfer energy between Cu$3d_{x^2-y^2}$ and O$2p_\sigma$ orbitals, $U_d$ is the on-site Coulomb interaction on Cu$3d_{x^2-y^2}$, and $U_p$ is the on-site Coulomb interactions on O$2p_\sigma$.

We calculate dynamical charge structure factor on O$2p_y$ orbital, $N_{2p_y}(\mathbf{q}, \omega)$, for the three-band Hubbard model (see the main text) by dynamical density-matrix renormalization group (DMRG) method. We use a $6 \times 4 = 24$ $CuO_2$ cluster with cylindrical geometry where the $x$ direction is of periodic boundary condition while the $y$ direction is of open boundary condition. In the cluster ($L_x = 6$ and $L_y = 4$), the $x$ component of momentum $\mathbf{q}$ is determined by using a usual translational symmetry, i.e., $q_x = n_x \pi / L_x$ ($n_x = 1, 2, \cdots, L_x$), but the $y$ component is given by $q_y = n_y \pi / (L_y + 1)$ ($n_y = 1, 2, \cdots, L_y$) because of open boundary condition. Defining $l_x$ ($l_y$) as the $x$ ($y$) component of O$2p_y$ site $l$, we define the charge operator for $2p_y$ orbitals as

$$
N^{2p_y}_{\mathbf{q}} = \sqrt{\frac{2}{L_x(L_y+1)}} \sum_l^L \sin(q_y l_y) e^{-i q_x l_x} n_l
$$

with $n_l$ being the number operator at site $l$.

In dynamical DMRG, we use a mutitarget scheme and one of the targets, $(\omega - H + E_0 + i\gamma)^{-1} N^{2p_y}_{\mathbf{q}} |0\rangle$, is evaluated by using a kernel-polynomial expansion method [3]. In our kernel-polynomial expansion method,

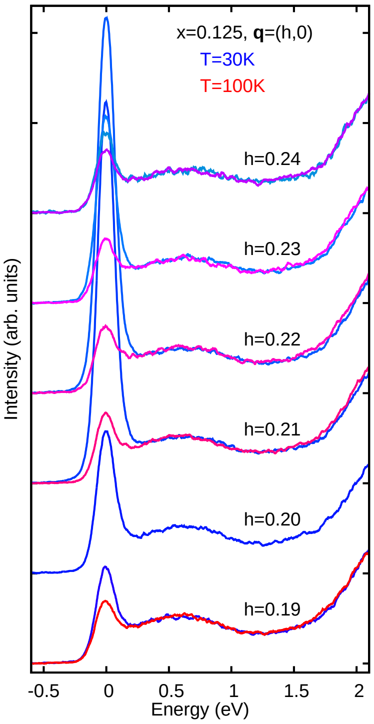


FIG. 3. (Color online) Oxygen $K$-edge RIXS spectra of $La_{2-x}Ba_xCuO_4$ ($x = 0.125$) measured below (30 K) and above (100 K) the transition temperature of charge order ($T_{co} = 50$ K).

the Lorentzian broadening is replaced by a Gaussian broadening with half width at half maximum 0.1 eV. In our numerical calculations, we divide the energy interval from 0 eV to 1.2 eV by 61-mesh points and have targeted all of the points at once.

To perform DMRG, we construct a snakelike one-dimensional chain, and use the truncation number $m = 2000$, and resulting truncation error is less than $2 \times 10^{-3}$. In order to check the accuracy of our results, we examine $m$ dependence of $N_{2p_y}(\mathbf{q}, \omega)$. Figure 2 shows the results for hole concentration $x = 1/12$ at $\mathbf{q} = (1/6, 1/10)$. The difference between $m = 1500$ and $m = 2000$ is small near the peak position, though the convergence is not perfect at higher energy region. Since it takes 24 hours by using 9600 nodes in the K computer, RIKEN Advanced Institute for Computational Science, to obtain a single curve of $N_{2p_y}(\mathbf{q}, \omega)$ with $m = 2000$ by our dynamical DMRG code, it is practically difficult to increase $m$ further more to perform systematic calculations of the doping and momentum dependence of dynamical charge structure factors.

## S3. TEMPERATURE DEPENDENCE OF O K-EDGE RIXS SPECTRA

We measured the oxygen $K$-edge RIXS spectra of of $La_{2-x}Ba_xCuO_4$ ($x = 0.125$) across the transition temperature of charge order at $T_{co} = 50$ K [4]. Figure 3 shows the spectra below (30 K) and above (100 K) $T_{co}$. Experimental condition is the same as the one of Fig. 2(b) in the main paper. While the charge order is confirmed by the enhanced elastic scattering at 30 K, an inelastic part does not charge across $T_{co}$.

* Present address: Department of Physics, Massachusetts Institute of Technology, Cambridge, MA 02139, USA


[1] K. Tsutsui and T. Tohyama, Phys. Rev. B **94**, 085144 (2016).

[2] K. Ishii, M. Fujita, T. Sasaki, M. Minola, G. Dellea, C. Mazzoli, K. Kummer, G. Ghiringhelli, L. Braicovich, T. Tohyama, K. Tsutsumi, K. Sato, R. Kajimoto, K. Ikeuchi, K. Yamada, M. Yoshida, M. Kurooka, and J. Mizuki, Nat. Commun. **5**, 3714 (2014).

[3] S. Sota and T. Tohyama, Phys. Rev. B **82**, 195130 (2010).

[4] M. Fujita, H. Goka, K. Yamada, J. M. Tranquada, and L. P. Regnault, Phys. Rev. B **70**, 104517 (2004).
